# Supplementary material for: On Differentially Private 3D Medical Image Synthesis with Controllable Latent Diffusion Models
Source: arXiv:2407.16405 source file (2024-07-23)
Supplement: Supplementary file 1 [file Appendix.tex]

\section{Conditioning attributes}

\begin{table}[h]
\centering
\caption{Summary Statistics for UKBB Dataset}
\label{tab:conditioning_attributes_summary_stats}
\begin{tabular}{@{}lcc@{}}
\toprule
\textbf{Attribute} & \textbf{Mean} & \textbf{Std} \\
\midrule
Age & 54.88 & 7.58 \\
Sex & 0.48 & 0.50 \\
\ac{BMI} & 26.52 & 4.39 \\
Phase (\ac{ES} or \ac{ED}) & 0.50 & 0.50 \\
Angle (of cardiac structure) & -0.14 & 26.12 \\
Depth ($\#$ non-padded slices) & 10.82 & 1.19 \\
LV \ac{ED} Volume & 155.70 & 37.13 \\
LV \ac{ES} Volume & 67.25 & 21.17 \\
LV Ejection Fraction & 57.22 & 6.39 \\
RV \ac{ED} Volume & 146.90 & 33.82 \\
RV \ac{ES} Volume & 60.02 & 19.32 \\
RV Ejection Fraction & 59.55 & 6.25 \\
Myocardial \ac{ES} Wall Thickness & 8.86 & 1.21 \\
Myocardial \ac{ED} Wall Thickness & 5.70 & 0.78 \\
\bottomrule
\end{tabular}
\end{table}

\section{VQ-VAE Results}

\begin{figure}
    \centering
    \includegraphics[width=\linewidth]{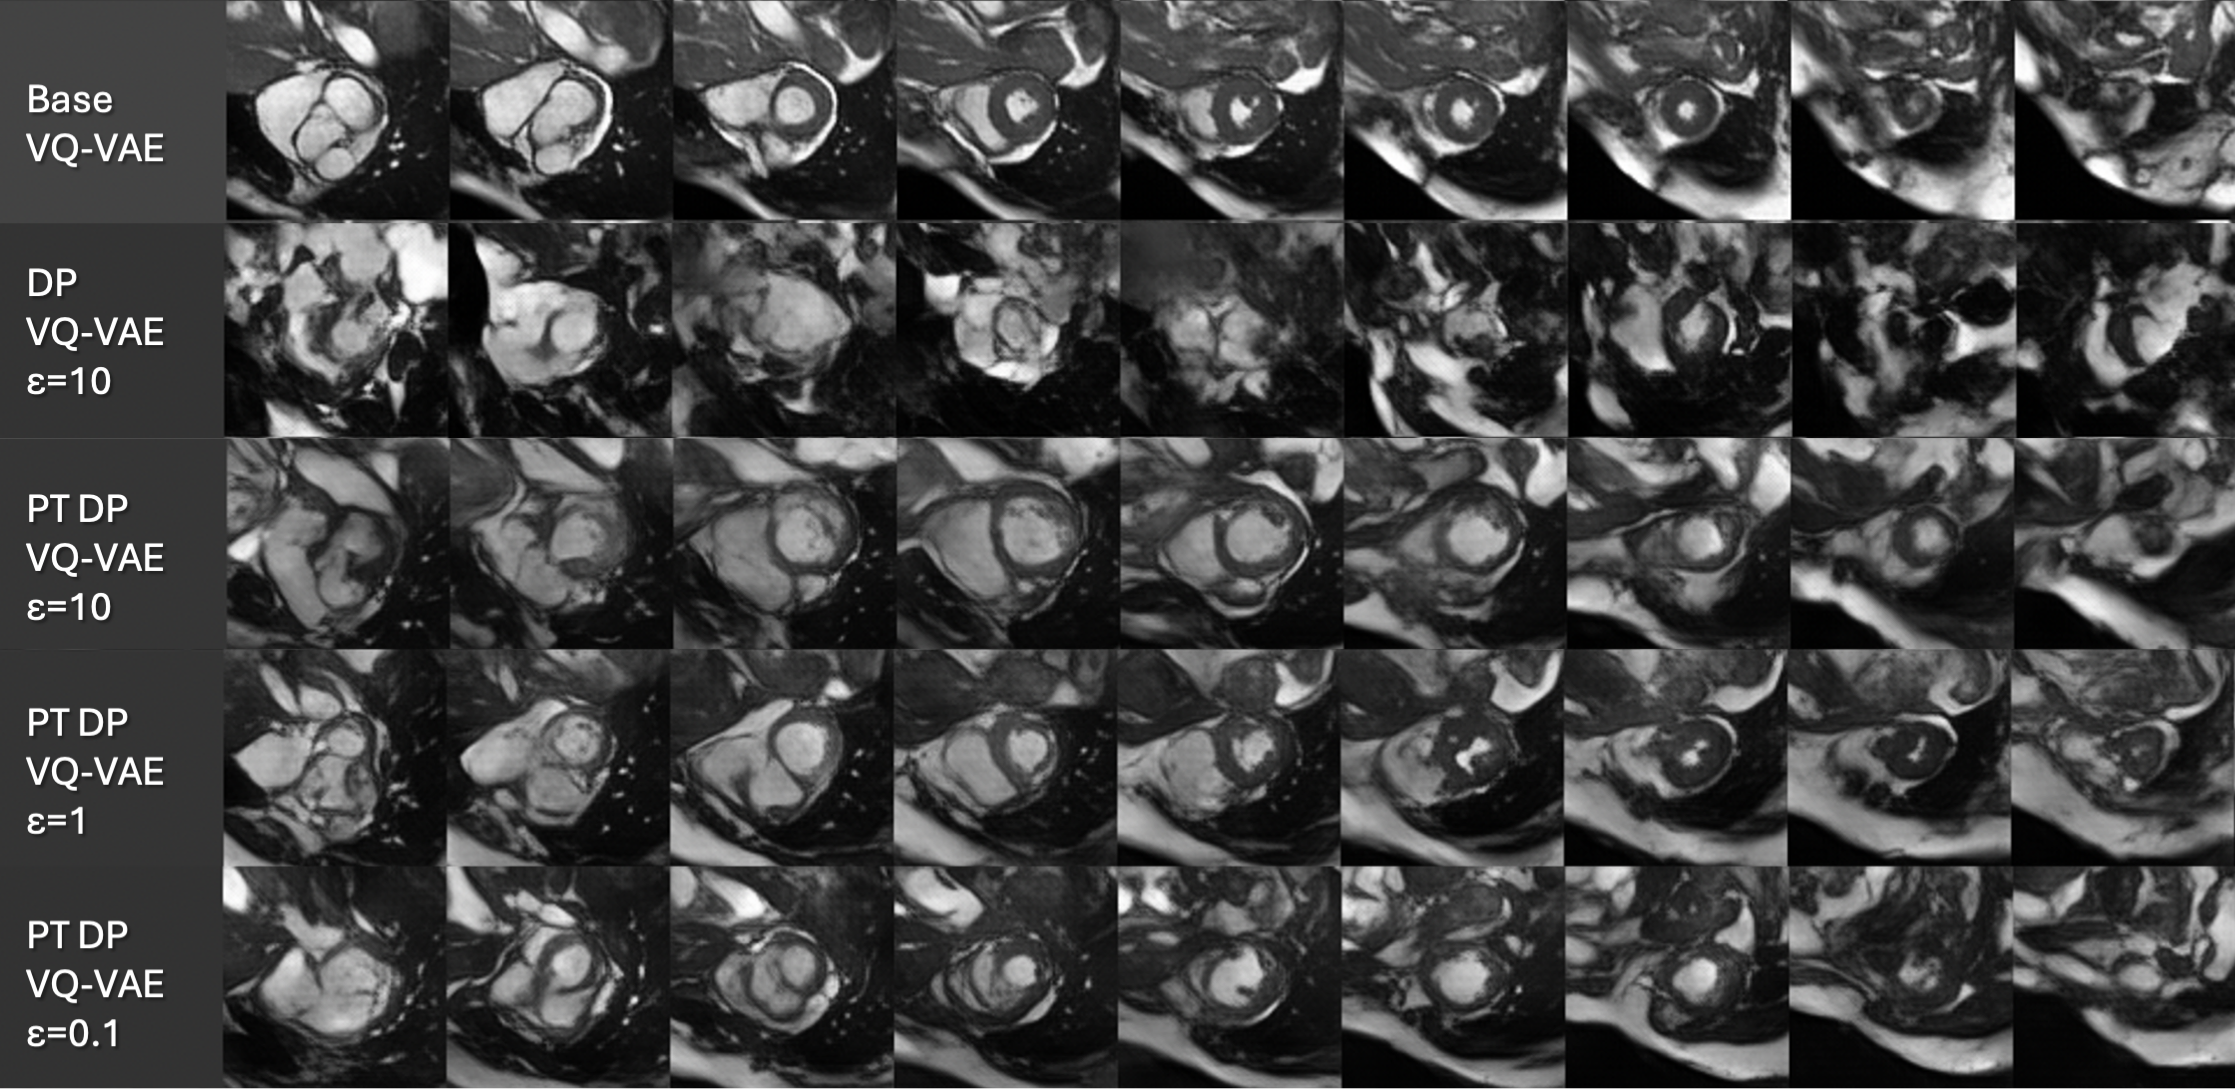}
    \caption{Synthetic 3D CMRI images at ES phase from VQ-VAE models with and without DP, PT and various privacy levels. From left to right: slices from the basal level to the apex.}
    \label{fig:GeneratedImagesVQ}
\end{figure}
